# Supplementary material for: Dynamics of a driven confined polyelectrolyte solution
Source: arXiv:2009.05656 source file (2020-09-11)
Supplement: Supplementary file 1 [file SIAppendix.pdf]

# Dynamics of a driven confined polyelectrolyte solution (Supplementary Information)

Debarshee Bagchi[1] and Monica Olvera de la Cruz[1,2,3,*]

[1]*Department of Materials Science and Engineering, Northwestern University, Evanston, IL 60208, United States*
[2]*Department of Chemical and Biological Engineering, Northwestern University, Evanston, IL 60208, United States*
[3]*Department of Physics and Astronomy, Northwestern University, Evanston, IL 60208, United States*

(Dated: August 25, 2020)

**MODEL-I: DIFFERENT ELECTRIC FIELDS: POLYELECTROLYTE AND COUNTERION MOBILITIES**

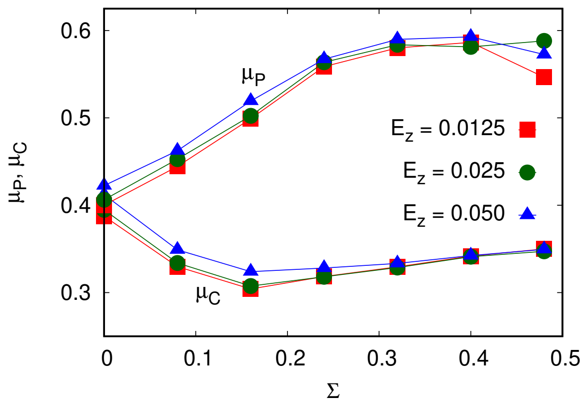


Figure S1. Polyelectrolyte mobility $\mu_P$ and counterion mobility $\mu_C$ for three different strengths of the external electric field. The mobilities, $\mu_P$ and $\mu_c$, change only slightly for the range of values we have chosen for $\vec{E}$. This shows that we are in the linear regime with respect to the external electric field.

**MODEL-I: COUNTERION SCREENING FOR DIFFERENT CONFINEMENT RADII**

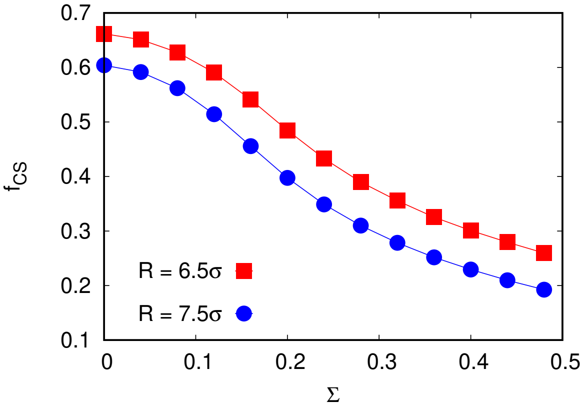


Figure S2. Counterion screening fraction $f_{CS}$ decreases as $\Sigma$ is increased. Counterion screening also decreases as the confinement radius increases.

## ELECTROLYTES: MONOVALENT AND MULTIVALENT

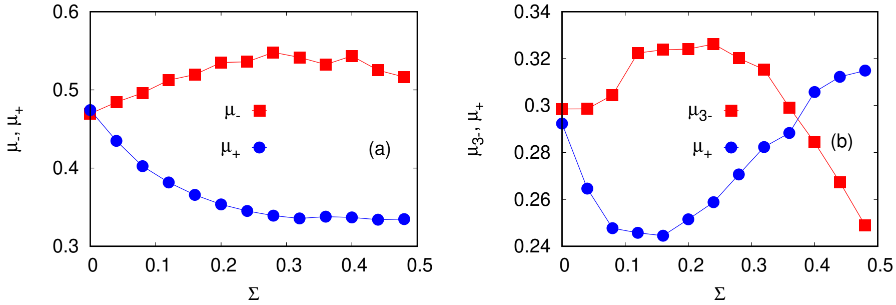


Figure S3. Mobilities of positive and negative ions for (a) electrolyte with monovalent cations and monovalent anions, and (b) electrolyte with monovalent cations and trivalent anions. The multivalent electrolyte shows pronounced non-monotonic variations with Σ. For case (b) the number of anions is one-third of the case (a) so as to maintain the same charge density inside the confinement.

## MODEL-I: POSITIVELY CHARGED CONFINEMENT OF DIFFERENT LENGTHS

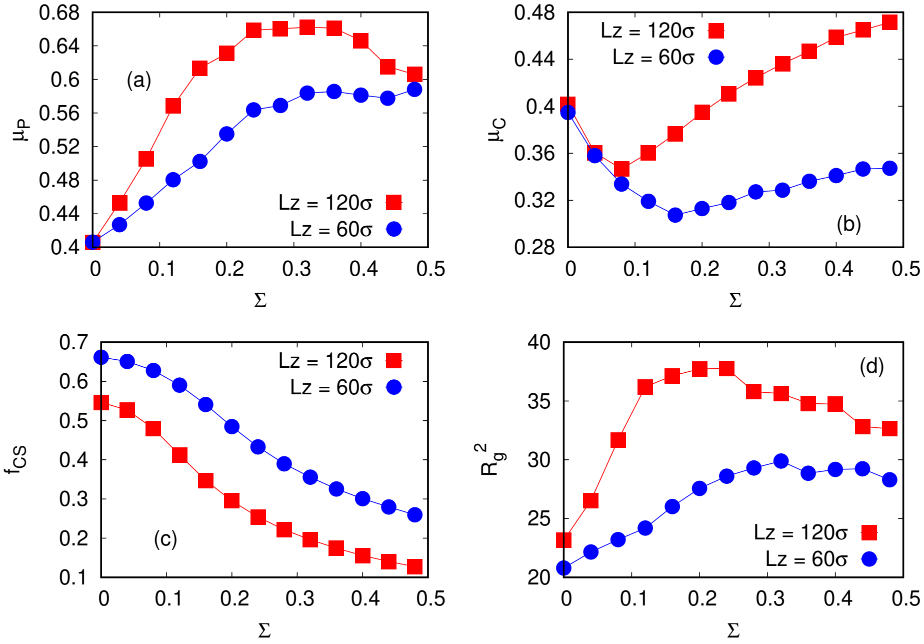


Figure S4. (a) Polyelectrolyte mobility $\mu_P$ and (b) counterion mobility $\mu_C$, for two confinements with different lengths $L_z = 60\sigma$ and $120\sigma$, and the same radius $R = 6.5\sigma$. (c) The fraction of counterions $f_{CS}$ screening the polyelectrolyte chains, and (d) the mean $R_g^2$ for the polyelectrolyte chains, both as a function of SCD Σ.

## MODEL-I: NEGATIVELY CHARGED CONFINEMENT: NET DENSITY

Unlike the positively charged confinement, for the case of a negatively charged confinement, the rearrangement of charges does not occur. This is shown in the series of color-maps in Fig. S5a representing the net density $\rho_{+} - rho_{-}$ inside the confinement. As a consequence, the counterion mobility increases monotonically as $\Sigma$ is increased from zero, as in Fig. S5b. The mobility of the polyelectrolyte chains is found to remain essentially unaltered, as can be seen in Fig. S5b. It seems that the counterions screen the charge on the confinement very effectively, and so the polyelectrolyte chains remain unaffected by the charged confinement.

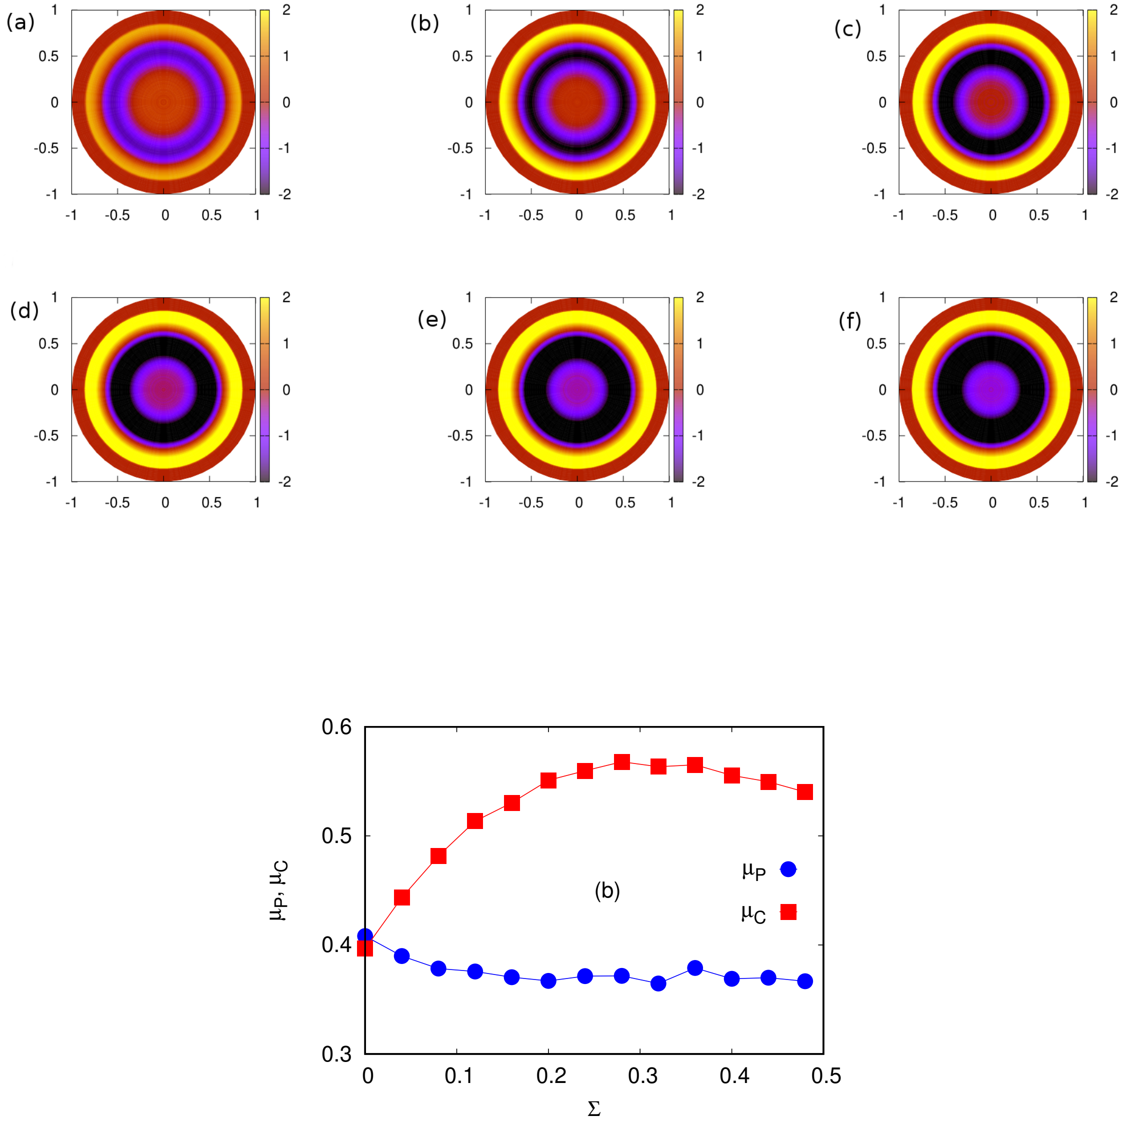


Figure S5. (a) Color-map of the net densities (normalized), for different values (magnitudes) of the surface charge density: from(a)–(f) $\Sigma = 0, 0.04, 0.08, 0.12, 0.16, 0.20\,C/m^2$. (b) Mobilities $\mu_P$ and $\mu_C$ with SCD $\Sigma$.

### MODEL-I: COUNTERION SCREENING FOR DIFFERENT POLYELECTROLYTE CHAIN LENGTHS

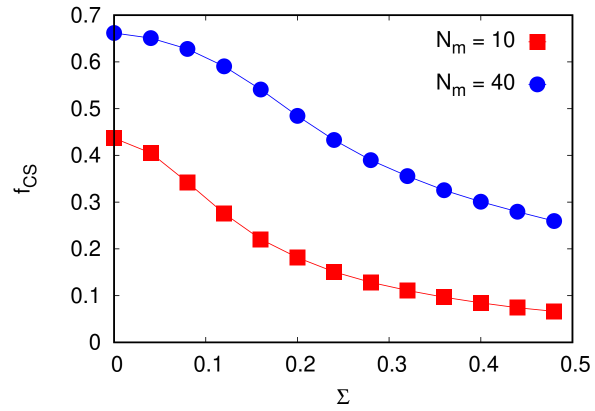


Figure S6. Counterion screening fraction $f_{CS}$ for two different values of $N_m$. The fraction $f_{CS}$ decreases as $N_m$ is decreased.

### MODEL-I: POLYELECTROLYTE SEPARATION IN A NEGATIVELY CHARGED CONFINEMENT

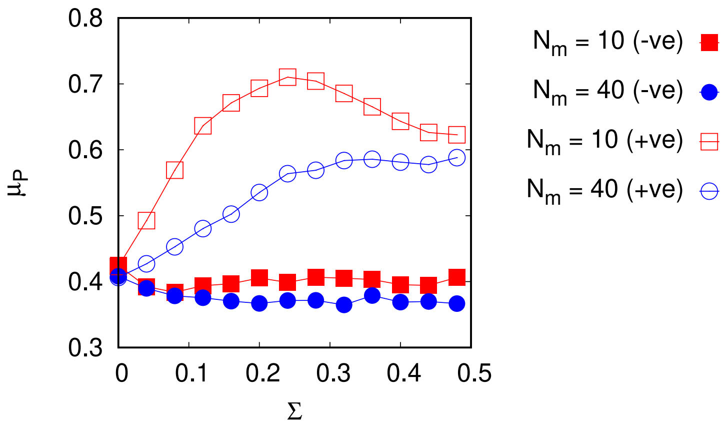


Figure S7. Comparison of polyelectrolyte separation in a negatively (-ve) charged confinement with a positively (+ve) charged one. The polyelectrolyte chains are negatively charged in both cases. The separation is much more efficient in the positively charged confinement due to the friction imparted by the oppositely charged confinement surface on the polyelectrolyte chains. For all the curves $N_c = 10$.

## MODEL-II: POSITIVELY CHARGED CONFINEMENT: NET DENSITY

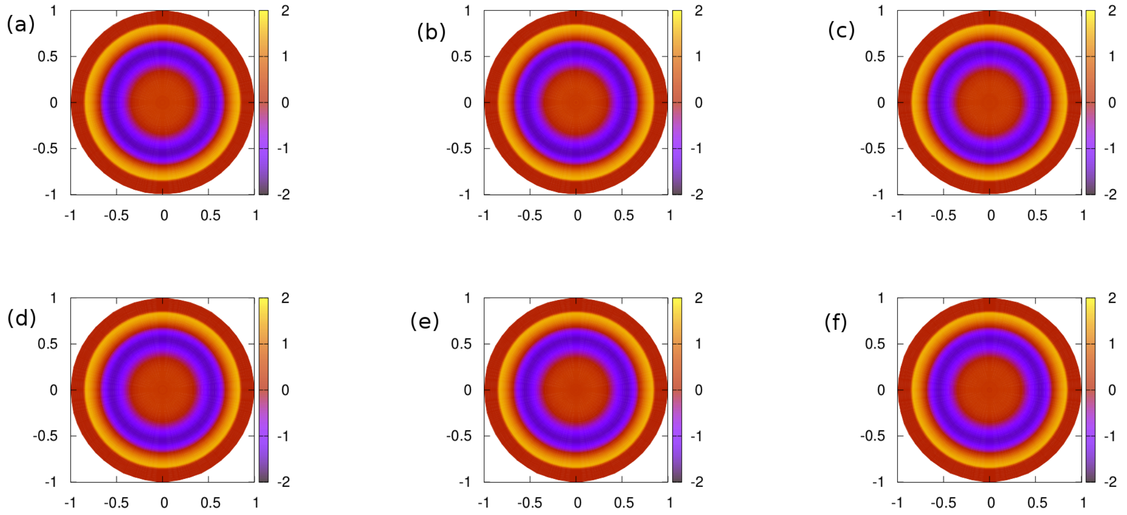


Figure S8. Color-map of the net density (normalized) inside the confinement for different surface charge density: from (a)–(f) $\Sigma = 0, 0.04, 0.08, 0.12, 0.16, 0.20\ C/m^2$, when the confinement counterions are outside (Model-II). The net density map does not change and is independent of the value of $\Sigma$. This shows why the mobilities, $\mu_P$ and $\mu_C$, are independent of $\Sigma$ for this case.

## MODEL-II: SIMULATIONS WITH AND WITHOUT INDUCED CHARGES

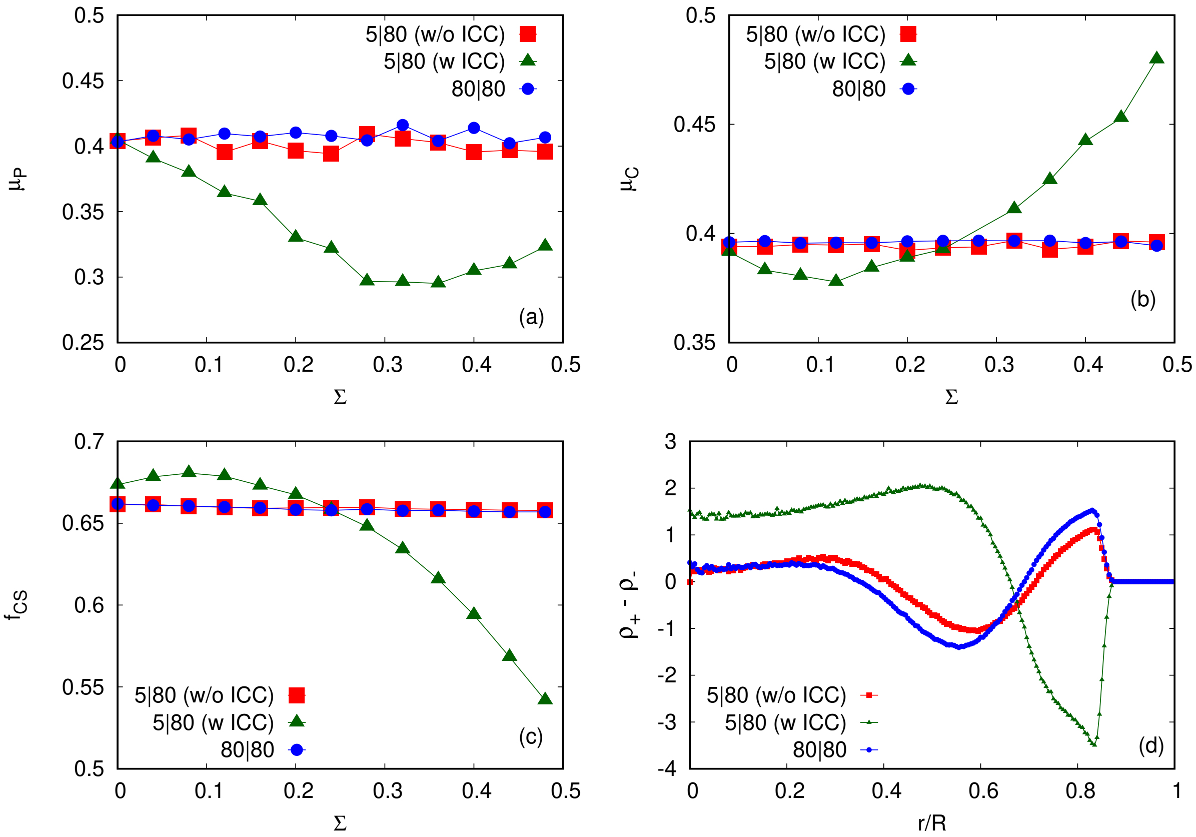


Figure S9. Model-II: (a) Polyelectrolyte mobility $\mu_P$ and (b) counterion mobility $\mu_C$, with induced charges (w ICC), without induced charges (w/o ICC), and without dielectric mismatch (80|80). Thus, even with a mismatch of dielectric constants, the mobility is independent of Σ if induced charges are not taken into account. In other words, this shows that the mobility of the polyelectrolyte chains does not depend on whether the confinement counterions are in a medium of dielectric constant $\varepsilon_1 = 5$ or $\varepsilon_1 = 80$, and their presence is experienced by the polyelectrolyte solution only *via* the induced charges. The counterion mobility can be explained straightforwardly from the counterion screening fraction $f_{CS}$ as shown in (c) for the three cases. In (d), we show the number density difference between the positive and the negative charges inside the confinement for $\Sigma = 0.40\ C/m^2$. As can be seen, in the presence of induces charges, the density profile (in nm$^{-3}$) changes drastically. The polyelectrolytes (negatively charged) are strongly attracted to the surface of the confinement and release the counterions which move away from the confinement. This enhanced attraction increases the friction between the polyelectrolyte and the confinement surface appreciably, that essentially leads to the enhanced polyelectrolyte separation in Model-II.

* E-mail address: m-olvera@northwestern.edu
